# Supplementary material for: Distributed Stochastic Optimization of a Neural Representation Network for Time-Space Tomography Reconstruction
Source: arXiv:2404.19075 source file (2025-02-26)
Supplement: Supplementary file 1 [file sec_supp.tex]

\section{Supplementary Document}

We use a Implicit Neural Representation (INR) network, 
$\mathcal{M}_{\gamma}$, to 
learn to predict the LAC, $\mu(x,y,z,t)$, from 
an encoding of the time-space coordinates $(x,y,z,t)$.
Here, $\gamma$ denotes the parameters (weights and bias terms)
of the INR network $\mathcal{M}_{\gamma}$.
We train the INR to predict $\mu(x,y,z,t)$ .
Thus, our objective is to solve the following optimization
problem,
\begin{equation}
\label{eq:lossmin}
\hat{\mu}\left(\cdot\right) = \arg\min_{\mu(\cdot)} 
\sum_{i,j,k} w_{i,j,k}\left(y_{i,j,k}-\hat{f}_{i,j,k}\left(\mu(\cdot)\right)\right)^2,
\end{equation}
where the sum is over all measurements
and $\mu(\cdot)$ is a function of the 
coordinates $[x,y,z,t]^T$.

\subsection{Bounding line integration}
To efficiently compute the line integral 
in equation \eqref{eq:parlineint},
we limit the range for $\delta$ such that
the world coordinates $[x,y,z]^T$ is 
inside the interior of the field-of-view (FOV)
that contain the object.
The equation for the cross-section area 
of a cylinder is given by,
\begin{equation}
    x^2 + y^2 \leq r^2,
\end{equation}
where $r$ is the radius of the cylindrical FOV. 
The rotated world coordinates for $(\delta, x_d, z_d)$ 
at view angle $\theta_k$ are 
$(x_{s,k}+\delta(x_{d,k}-x_{s,k}))$ and 
$(y_{s,k}+\delta(y_{d,k}-y_{s,k}))$ 
along the $x$-axis and $y$-axis respectively.
Then, we can bound $\delta$ by solving the 
quadratic equation given below,
\begin{equation}
    (x_{s,k}+\delta(x_{d,k}-x_{s,k}) - x_{s0})^2 + 
    (y_{s,k}+\delta(y_{d,k}-y_{s,k}))^2 \leq r^2,
\end{equation}
where $x_{s0}$ is the center of rotation along the $x$-axis.
Substituting equations \eqref{eq:rotxsk}, \eqref{eq:rotysk},
\eqref{eq:rotxdk}, and \eqref{eq:rotydk}, we get,
\begin{multline*} 
(x_s \cos\left(\theta_k\right) - 
y_s \sin\left(\theta_k\right) - 
x_{s0}\cos\left(\theta_k\right)
+\delta((x_d-x_s) \cos\left(\theta_k\right) - 
(y_d-y_s) \sin\left(\theta_k\right)))^2 + \\
(x_s \sin\left(\theta_k\right) 
+ y_s \cos\left(\theta_k\right)
- x_{s0}\sin\left(\theta_k\right)
+ \delta((x_d-x_s) \sin\left(\theta_k\right) 
+ (y_d-y_s) \cos\left(\theta_k\right)))^2 \leq r^2
\end{multline*}
Next, we collect all terms associated with 
the sines and cosines as shown below,
\begin{multline*} 
\left(\cos\left(\theta_k\right)
\left(x_s-x_{s0}+\delta(x_d-x_s)\right)
+ \sin\left(\theta_k\right)
\left(-y_s-\delta(y_d-y_s)\right)\right)^2 \\
+ \left(\cos\left(\theta_k\right)
\left(y_s+\delta(y_d-y_s)\right)
+\sin\left(\theta_k\right)
\left(x_s-x_{s0}+\delta(x_d-x_s)\right)\right)^2 
\leq r^2.
\end{multline*}
After expanding the quadratic in the above equation,
we see that the equation is independent of $\theta_k$
as shown below,
\begin{equation}
\left(x_s-x_{s0}+\delta(x_d-x_s)\right)^2 +
\left(y_s+\delta(y_d-y_s)\right)^2 \leq r^2.
\end{equation}
After further expansion of the above quadratic,
we get,
\begin{multline}
\label{eq:solvquaddelta}
    \delta^2\left(\left(x_d-x_s\right)^2+\left(y_d-y_s\right)^2\right)
    + 2\delta \left(\left(x_s-x_{s0}\right)\left(x_d-x_s\right)+y_s\left(y_d-y_s\right)\right)+\\
    \left((x_s-x_{s0})^2+y_s^2-r^2\right) \leq 0.
\end{multline}
The limits on $\delta$ for integrating within the cylindrical 
FOV of the object in Fig. \ref{fig:geomdiag} is obtained by 
solving equation \eqref{eq:solvquaddelta}.
Let $a=\left(x_d-x_s\right)^2
+\left(y_d-y_s\right)^2$, 
$b=2\left(\left(x_s-x_{s0}\right)\left(x_d-x_s\right)+y_s\left(y_d-y_s\right)\right)$,
and $c=(x_s-x_{s0})^2+y_s^2-r^2$.
Then, the roots of the equation \eqref{eq:solvquaddelta} are,
\begin{align}
    \delta_{min} = \frac{-b-\sqrt{b^2-4ac}}{2a}, \text{ and }
    \delta_{max} = \frac{-b+\sqrt{b^2-4ac}}{2a}.
    \label{eq:deltaminmax}
\end{align}

\subsection{Cone-Beam Geometry}
For cone-beam, the source is located at a distance 
of $SOD$ (source-to-object distance) to the left 
of the object.
Hence, the coordinates of the X-ray source are
$x_s=0$, $y_s=-SOD$, and $z_s=0$.
Similarly, the detector is located at a distance
of $ODD$ (object-to-detector distance) to the right
of the object.
To compute the forward model term 
$f_{i,j,k}(\mu(\cdot))$ in \eqref{eq:estforwmod}, 
we substitute $x_s=0$, $y_s=-SOD$, $z_s=0$, and $y_d=ODD$
in equations \eqref{eq:deltaminmax}, \eqref{eq:rotxsk},
\eqref{eq:rotysk}, \eqref{eq:rotxdk}, \eqref{eq:rotydk},
and \eqref{eq:estforwmod}.
The lower and upper bounds for $\delta$ are obtained
by substituting $a=x_s^2+(ODD+SOD)^2$, 
$b=-2(x_{s0}x_d+SOD(ODD+SOD))$, and 
$c=x_{s0}^2+SOD^2-r^2$ in equation \eqref{eq:deltaminmax}.
The arc-length parameter, $s(\cdot)$, in \eqref{eq:estforwmod} 
is $\sqrt{x_d^2+(ODD+SOD)^2+z_d^2}$.

\section{Forward Model}
In a X-ray CT scanner, 
the propagation direction of X-rays 
is defined by the so-called geometry of the scanner, 
which is a function of the position and orientations 
of the X-ray source and detection system.
We consider three X-ray scanner geometries 
including cone-beam, fan-beam, and 
parallel-beam geometry.
For the detector, 
we use a scintillator-based detection 
system that is modeled as a 2D panel consisting
of a rectilinear grid of sensor pixels 
with finite area. 

\begin{figure}[!thb]
\begin{center}
\includegraphics[width=4in]{figs/geometry.png}
\end{center}
\caption{\label{fig:geomdiag}
}
\end{figure}

\begin{figure}[!thb]
\begin{center}
\includegraphics[width=4.5in]{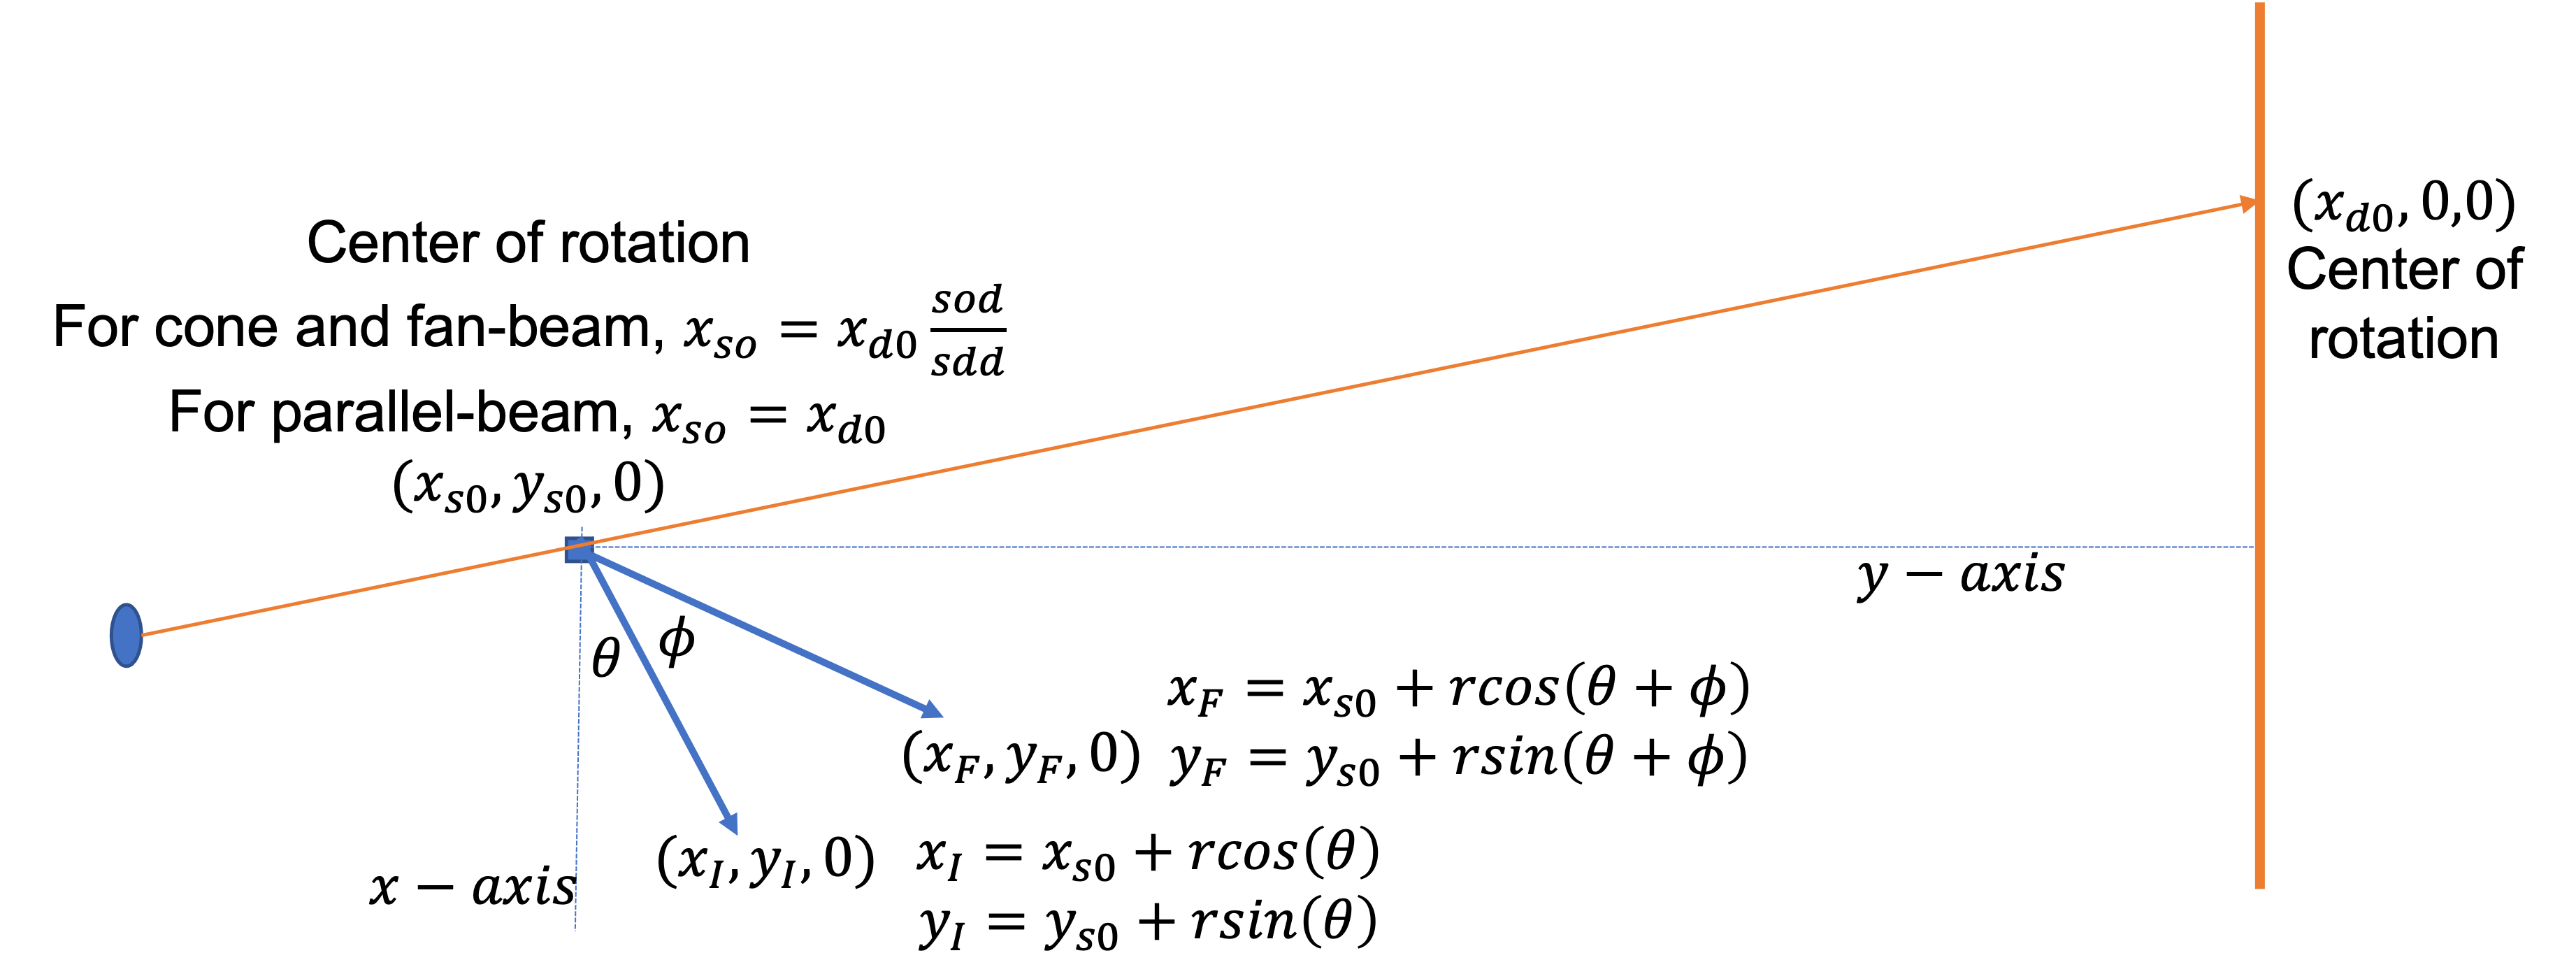}
\end{center}
\caption{\label{fig:rotdiag}
}
\end{figure}

The measured CT data is a function of the time-space 
distribution of the linear attenuation coefficient 
(LAC), denoted by $\mu([t,z,y,x]^T)$, of the object.
Here, $t$, $z$, $y$, and $x$ are the time, 
$z$-axis, $y$-axis, and $x$-axis world 
coordinates respectively.
The LAC is a measure of the amount of X-ray
attenuation caused by various material
interaction properties such as photoelectric
absorption and scatter. 
For any detector pixel indexed by $(i,j)$,
the measurement is an average of the 
X-ray intensities along a continuum 
of rays that originate from the 
point-source, propagate through the object, and
end at a location inside the 
pixel's surface area.
Here, the row and column indices of a 
detector pixel are denoted by 
$i$ and $j$ respectively. 
Let the set of all coordinates within the 
surface area of the detector pixel $(i,j)$
be given by,
\begin{multline}
    C_{i,j} = \left\lbrace (x_d, z_d) \,\vert\, 
    -C_x + i\Delta_x \leq x_d < -C_x + (i+1)\Delta_x,\right.\\
    \left. -C_z + j\Delta_z \leq z_d < -C_z + (j+1)\Delta_z
    \right\rbrace,
\end{multline}
where $x_d$ and $z_d$ are the $x$-axis 
and $z$-axis coordinates on the detector plane,
and $\Delta_x$ and $\Delta_z$ are the widths 
of the detector pixel along the $x$-axis 
and $z$-axes respectively.
Here, $C_x$ and $C_z$ are the distances
of the optical axis from the left-vertical and 
bottom-horizontal edges of the detector panel. 

The measurement made by detector pixel $(i,j)$
is a direct measure of the linear projections 
of the LAC $\mu([x,y,z,t]^T)$ along rays that
connect the X-ray source to points on the
surface of the pixel $(i,j)$.
The $y$-axis is defined along the optical axis, 
which is the ray originating at the X-ray source
and intersecting perpendicularly at the detector.
Without loss of generality, 
the $x$-axis coordinate for the optical axis
is $x=0$ and $y=0$ is the center of 
rotation for the object along the $y$-axis.
The center of rotation for the object
along the $x$-axis is denoted by $x_{s0}$.
The object is rotated along the $z$-axis
and $z=0$ marks the center of the object
along the $z$-axis. 
To rotate the source and detector coordinates
in the $x-y$ axial plane by an 
anti-clockwise angle of $\theta_k$, we use the 
following equations,
\begin{align}
    x_{s,k} & = x_s \cos\left(\theta_k\right) - y_s \sin\left(\theta_k\right) + \left(x_{s0} -
      x_{s0}\cos\left(\theta_k\right)\right),  \label{eq:rotxsk}\\
    y_{s,k} & = x_s \sin\left(\theta_k\right) 
      + y_s \cos\left(\theta_k\right)
      - x_{s0}\sin\left(\theta_k\right), \label{eq:rotysk}\\
    x_{d,k} & = x_d \cos\left(\theta_k\right) - y_d \sin\left(\theta_k\right) + \left(x_{s0} -
      x_{s0}\cos\left(\theta_k\right)\right), \text{ and } \label{eq:rotxdk} \\
    y_{d,k} & = x_d \sin\left(\theta_k\right) 
      + y_d \cos\left(\theta_k\right)
      - x_{s0}\sin\left(\theta_k\right).\label{eq:rotydk}
\end{align}
Anti-clockwise rotation of source and detectors 
by an angle of $\theta_k$ is equivalent to clockwise
rotation of object coordinates by $\theta_k$.

The linear projection of the LAC, $\mu(\cdot)$, 
along a ray that connects
the X-ray source at $[x_s, y_s, z_s]^T$ and 
a detector coordinate at $[x_d, y_d, z_d]^T$ 
at time $t=t_k$ is,
\begin{multline}
    p\left(\begin{bmatrix}
    x_d \\ y_d \\ z_d
    \end{bmatrix},
    \begin{bmatrix}
    x_s \\ y_s \\ z_s
    \end{bmatrix}, 
    \begin{bmatrix}
    t_k \\
    \theta_k
    \end{bmatrix}
    \right) =
    \int_{\delta=\delta_{min}}^{\delta_{max}} 
    s\left(\begin{bmatrix}
    x_d\\ y_d \\ z_d
    \end{bmatrix},
    \begin{bmatrix}
    x_s\\ y_s \\ z_d
    \end{bmatrix}\right)\\
    \mu\left(\begin{bmatrix}
    x_{s,k} \\ y_{s,k} \\ z_s \\ t_k
    \end{bmatrix}
    + \delta
    \begin{bmatrix}
    x_{d,k}-x_{s,k} \\ 
    y_{d,k}-y_{s,k} \\ 
    z_d-z_s \\
    0
    \end{bmatrix}\right)
    d\delta,
    \label{eq:parlineint}
\end{multline}
where $\delta$ is used to parameterize 
the line connecting 
$[x_s,y_s,z_s]^T$ and $[x_d,y_d,z_d]^T$.
The limits of the integral, 
$\delta_{min}$ and $\delta_{max}$,
mark the outer boundary of the object.
Thus, the LAC is zero for 
$\delta<\delta_{min}$ or $\delta>\delta_{max}$.
We assume that the object is stationary for the 
duration of the detector's exposure time. 
The arc-length is given by,
\begin{equation}
\label{eq:arclength}
s\left(\begin{bmatrix}
    x_d\\ y_d \\ z_d
    \end{bmatrix},
    \begin{bmatrix}
    x_s\\ y_s \\ z_d
    \end{bmatrix}\right) 
    = \left\vert\left\vert
    \begin{bmatrix}
    x_d\\ y_d \\ z_d
    \end{bmatrix}
    - \begin{bmatrix}
    x_s\\ y_s \\ z_s
    \end{bmatrix}
    \right\vert\right\vert^2_2.
\end{equation}
The source-to-object distance is 
$\vert y_s \vert$
and object-to-detector distance is 
$\vert y_d \vert$.

For each $(i,j,k)$, we compute several 
line integrals using equation \eqref{eq:parlineint} 
along the lines that connect the X-ray source 
to several locations on the finite sized 
detector pixel and average the line integrals
within each pixel. 
The measurement at detector pixel $(i,j)$ is,
\begin{equation}
\label{eq:beerstransavg}
    I_{i,j,k} = I^{(0)}_{i,j,k}\int_{(x_d,z_d)\in C_{i,j}}
    \exp\left\lbrace
    -p\left(\begin{bmatrix}
    x_d \\ y_d \\ z_d
    \end{bmatrix},
    \begin{bmatrix}
    x_s \\ y_s \\ z_s
    \end{bmatrix}, 
    \begin{bmatrix}
    t_k \\
    \theta_k
    \end{bmatrix}\right)
    \right\rbrace
    dx_d dz_d,\\
\end{equation}
where $I^{(0)}_{i,j,k}$ is the X-ray intensity 
in the absence of the object.
We approximate equation \eqref{eq:beerstransavg}
by moving the integration to within the exponential,
which is useful to formulate a linear forward model
that reduce the computational cost. 
Thus, our model for the measurement is,
\begin{equation}
\label{eq:beersattenavg}
    I_{k,i,j} = I^{(0)}_{k,i,j}\exp
    \left(-\int_{(x_d,z_d)\in C_{i,j}}
    p\left(\begin{bmatrix}
    x_d \\ y_d \\ z_d
    \end{bmatrix},
    \begin{bmatrix}
    x_s \\ y_s \\ z_s
    \end{bmatrix}, 
    \begin{bmatrix}
    t_k \\
    \theta_k
    \end{bmatrix}\right)
    dx_d dz_d\right).\\
\end{equation}

Our goal is to reconstruct $\mu([x,y,z,t]^T)$ from 
measurements $I_{i,j,k}$ using 
equation \eqref{eq:beersattenavg}.
Since equation \eqref{eq:beersattenavg} is non-linear, 
we use logarithms to obtain a relation that is 
linear in $\mu([x,y,z,t]^T)$.
Let $f_{i,j,k}\left(\mu(\cdot)\right)$ be the negative 
logarithm of the ratio between $I_{i,j,k}$ and $I_0(i,j,k)$.
Then, using the logarithmic transformation for 
equation \eqref{eq:beersattenavg}, we get,
\begin{multline}
\label{eq:logbeerslaw}
f_{i,j,k}\left(\mu\left(
\begin{bmatrix}
x\\ y\\ z\\ t
\end{bmatrix}
\right)\right) 
    =-\log\left\lbrace\frac{I_{i,j,k}}{I^{(0)}_{i,j,k}}\right\rbrace = \\
    \int_{(x_d,z_d)\in C_{i,j}}
    p\left(\begin{bmatrix}
    x_d \\ y_d \\ z_d
    \end{bmatrix},
    \begin{bmatrix}
    x_s \\ y_s \\ z_s
    \end{bmatrix}, 
    \begin{bmatrix}
    t_k \\
    \theta_k
    \end{bmatrix}\right)
    dx_d dz_d.
\end{multline}
In practice, we cannot measure $I^{(0)}_{i,j,k}$ at every $t_k$.
Instead, we acquire X-ray images without the object
at a few distinct time intervals and approximate 
$I^{(0)}_{i,j,k}$ from these images. 
Thus, the forward measurement model is,
\begin{equation}
\label{eq:forwmod}
y_{i,j,k} = f_{i, j, k}\left( 
\mu\left(\left[x, y, z,
t\right]^T\right)\right)
+ n_{i,j,k},
\end{equation}
where $n_{i,j,k}$ Poisson-like noise that 
is modeled as a Gaussian random variable with a
standard deviation of 
$\sqrt{f_{i, j, k}\left(\mu(\cdot)\right)}$.

To compute $f_{i,j,k}(\cdot)$, 
we need to numerically evaluate the integrals
in equations \eqref{eq:beersattenavg} 
and \eqref{eq:parlineint}.
For numerical integral calculation, 
we choose between either a regular equi-spaced 
sampling or randomized sampling for
$\delta$, $x_d$, and $z_d$.
For equi-spaced sampling, we regularly 
sample the detector coordinates
$(x_d, z_d) \in C_{i,j}$ with equal spacing
between adjacent samples along both $x$-axis and $z$-axis.
For each sampled $(x_d, z_d)$, we again perform 
equi-spaced sampling of the $\delta$ coordinate 
that parameterizes the line connecting the 
source to the detector pixel $(i,j)$.
For randomized sampling, we sample all the coordinates
of $\delta$, $x_d$, and $z_d$ uniformly at random.
Let $\Psi_{i,j,k}$ be the set of all sampled $(x_d, z_d, \delta)$
coordinates for the measurement at $(i,j,k)$.
Then, a numerical estimate for $f_{i,j,k}(\cdot)$
is given by,
\begin{multline}
    \hat{f}_{i,j,k}\left(\mu\left(
    \begin{bmatrix}
    x\\ y\\ z\\ t
    \end{bmatrix} \right)\right) =
    \frac{\left(\delta_{max}-\delta_{min}\right)}{\left\vert\Psi_{i,j,k}\right\vert}
    \sum_{(x_d,z_d,\delta)\in \Psi_{i,j,k}}
     s\left(\begin{bmatrix}
    x_d\\ y_d \\ z_d
    \end{bmatrix},
    \begin{bmatrix}
    x_s\\ y_s \\ z_d
    \end{bmatrix}\right)\\
    \mu\left(\begin{bmatrix}
    x_{s,k} \\ y_{s,k} \\ z_s \\ t_k
    \end{bmatrix}
    + \delta
    \begin{bmatrix}
    x_{d,k}-x_{s,k} \\ 
    y_{d,k}-y_{s,k} \\ 
    z_d-z_s \\ 0
    \end{bmatrix}\right).
    \label{eq:estforwmod}
\end{multline}
To compute $\hat{f}_{i,j,k}(\mu(\cdot))$, 
the limits for sampling of $x_d$, $z_d$, and $\delta$ 
are $\left(-C_x+i\Delta_x, -C_x+(i+1)\Delta_x\right)$,
$\left(-C_z+j\Delta_z, -C_z+(j+1)\Delta_z\right)$, and
$\left(l_{min}, l_{max}\right)$.
In equation \eqref{eq:estforwmod}, the summation
is over all the sampled values of $(x_d, z_d, \delta)$
in the region that connects the X-ray source source
to the surface area of the pixel $(i,j)$ 
at rotation angle $\theta_k$.
The samples of coordinates within this region 
for our integration by summation approach
is contained in the set $\Psi_{i,j,k}$.
In the next section, we substitute the LAC term,
$\mu(\cdot)$ in equation \eqref{eq:estforwmod}
with the neural representation 
network $\mathcal{M}_{\gamma}(\cdot)$.
Both $\mu(\cdot)$ and $\mathcal{M}_{\gamma}(\cdot)$
are functions of the world coordinates $(x,y,z,t)$.

\begin{figure}[t!]
  \centering
  \begin{subfigure}[t]{0.5\textwidth}
    \centering
    \includegraphics[width=0.99\textwidth]{figs/figure_MPM_128_psnr.png}
    \caption{Peak signal-to-noise ratio (PSNR)}
  \end{subfigure}%
  ~
  \begin{subfigure}[t]{0.5\textwidth}
    \centering
    \includegraphics[width=0.99\textwidth]{figs/figure_MPM_128_ssim.png}
    \caption{Structural Similarity Index (SSIM)}
  \end{subfigure}
  \caption{Quantitative evaluation of the MPM-simulated datasets using two image metrics between the reconstructed and the original ground-truth volume frames. $128\times128\times128\times181$. }
\end{figure}

\begin{figure}[!thb]
\begin{center}
\includegraphics[width=\textwidth]{figs/figure_MPM_128_results.pdf}
\end{center}
\caption{Reconstructed volume frames of the MPM-simulated datasets using the proposed method. $128\times128\times128\times181$. First, middle and last frames. }
\end{figure}
